# Supplementary material for: Shape Back-Projection In 3D Scenes
Source: arXiv:2101.06409 source file (2021-01-16)
Supplement: Supplementary file 1 [file appendix.tex]

\appendices

%Statistical Outlier Rejection
%\section{}
%\label{appendix_outlier_test}

%Moving Least Squares
%\section{}
%\label{appendix_mls}
